# Supplementary material for: FLEX: Feature Importance from Layered Counterfactual Explanations
Source: arXiv:2511.11891 source file (2025-11-14)
Supplement: Supplementary file 1 [file app0A.tex]

%
% file: localoperator.tex
% author: Victor Brena
% description: Briefly describes properties of the local operator.
%

\chapter{Appendix A}
\label{app:app01}

Begins an appendix

\
